# Supplementary material for: LIGO-PINN: Learned Initialization via Gated Optimization to Alleviate Convergence Failures in Physics Informed Neural Networks
Source: arXiv:2607.14233 source file (2026-07-15)
Supplement: Supplementary file 1 [file A5.Computation.tex]

\subsection{Computational Resource}\label{appendix:computation-resource}
All experiments were performed on a Linux server with an RTX A6000 GPU with 48GB vRAM.
To ensure reproducibility, we document the hardware and software environments used, as well as the approximate runtimes for our main experiments in Table~\ref{tab:comp_resources_specs}.

\small
\begin{table}[ht]
  \centering
  \caption{Hardware and Software Specifications}
  \label{tab:comp_resources_specs}
  \begin{tabular}{|l|l|}
    \hline
    \textbf{Component}          & \textbf{Specification}                       \\ \hline
    GPU                         & NVIDIA RTX A6000 (48 GB VRAM)               \\ \hline
    CPU                         & Intel(R) Xeon(R) Platinum 8358 CPU @ 2.60GHz \\ \hline
    System RAM                  & 2 TB DDR4                                 \\ \hline
    Operating System            & Ubuntu 20.04 LTS                            \\ \hline
    Python                      & 3.10                                         \\ \hline
    PyTorch                     & 2.4 (CUDA 12)                          \\ \hline
    Experiment Tracking         & MLflow 2.14                              \\ \hline
  \end{tabular}
\end{table}

\paragraph{Computation Cost.} 
To provide a holistic context regarding the compute cost of the initialization strategy, 
we report wall-clock training time (in minutes) and peak GPU memory usage (in MB) 
in Table~\ref{tab:computation_cost}. All measurements were conducted on an NVIDIA RTX A6000 GPU (48\,GB vRAM) to ensure consistency 
 Peak memory usage was measured using \texttt{nvidia-smi}. 

\begin{table}[ht]
\small
\caption{Computation cost for 1D Convection system. We report wall-clock training time (minutes) and peak memory (MB).}
\label{tab:computation_cost}
\centering
\begin{tabular}{lcc}
\toprule
\textbf{Stage / Method} & \textbf{Time (min)} & \textbf{Peak GPU Memory (MB)} \\
\midrule
LIGO-PINN (Invariance Encoding) & 3.1  & 740 \\
LIGO-PINN (Fine-Tuning)         & 10.4 & 540 \\
Xavier Init. PINN Training      & 10.4 & 540 \\
\bottomrule
\end{tabular}
\end{table}

We emphasize that the meta-training stage (invariance encoding) is a \emph{one-time cost}. 
Once the initialization is learned, it can be reused across multiple PDE tasks in the same domain class, 
thereby amortizing this overhead. Furthermore, the collocation points and grid resolution were kept 
constant between the invariance encoding and task-specific fine-tuning stages. These results confirm 
that \mymethod{} scales comparably to standard PINNs in terms of grid resolution, with the only 
additional overhead being the upfront, one-time meta-training stage.
