# Supplementary material for: LIGO-PINN: Learned Initialization via Gated Optimization to Alleviate Convergence Failures in Physics Informed Neural Networks
Source: arXiv:2607.14233 source file (2026-07-15)
Supplement: Supplementary file 2 [file experiment_setup.tex]

\begin{table}[htbp]
\centering
\caption{Summary of Experimental Setup}
\begin{tabular}{p{4.5cm} p{9cm}}
\toprule
\textbf{Component} & \textbf{Details} \\
\midrule
\textbf{System Description} & 1D convection equation \\
\textbf{Neural Network Architecture} & 
Input: \(x, t\) (2D) \newline
Hidden Layers: 4 layers with 50 neurons each \newline
Activation: \texttt{Tanh} \newline
Output: \(\hat{u}\) (1D) \newline
Initialization: Kaiming \\
\textbf{Training Configuration} &
Epochs: 40,000 \newline
Boundary/Data Points: 1,000 \newline
Optimizer: Adam \newline
Learning Rate: 0.005 (cosine annealing) \newline
Domain: \(x \in [0, 2\pi],\; t \in [0,1]\) \\
\textbf{Meta-Learning Configuration} &
Meta Steps: 200 \newline
Inner Steps per Task: 20 \newline
Tasks (\(\beta\)): [5, 10, 15, 20, 25] \newline
Tasks per Meta-step: 3 \\
\textbf{Evaluation Tasks} &
Interpolation: \(\beta = 7.5, 12.5, 17.5, 22.5\) \newline
Extrapolation: \(\beta = 30, 40, 50, 60, 70, 80\) \\
\textbf{Loss \& Hyperparameters} &
\(\mathcal{L}_{total} = \lambda_{r}\mathcal{L}_{r} + \lambda_{d}\mathcal{L}_{d}\) \newline
\(\lambda_{r} = 0.005,\quad \lambda_{d} = 1.0\) \\
\bottomrule
\end{tabular}
\label{tab:heat-exp-setup}
\end{table}

\begin{table}[htbp]
\centering
\caption{Experimental Setup for 2D Helmholtz System}
\begin{tabular}{p{4.5cm} p{9cm}}
\toprule
\textbf{Component} & \textbf{Details} \\
\midrule
\textbf{System Description} &
2D Helmholtz equation: \( \Delta u + k^2 u = f(x, y) \) \newline
\( k^2 = a_1^2 + a_2^2 \), \( a_1 = 1 \), \( a_2 \in [1, 2, 3, 4, 5] \) \newline
Domain: \( (x_1, x_2) \in [-1, 1]^2 \) \\
\textbf{Neural Network Architecture} & 
Input: \(x_1, x_2\) (2D) \newline
Hidden Layers: 4 layers with 50 neurons each \newline
Activation: \texttt{Tanh} \newline
Output: \(\hat{u}\) (1D) \newline
Initialization: Xavier \\
\textbf{Training Configuration} &
Epochs: 40,000 \newline
Boundary/Data Points: 1,000 (each for boundary and interior) \newline
Optimizer: Adam \newline
Learning Rate: 0.005 (cosine annealing) \newline
Domain Sampling: \(x_1, x_2 \in [-1, 1]\) \\
\textbf{Meta-Learning Configuration} &
Meta Steps: 200 \newline
Inner Steps per Task: 10 \newline
Tasks per Meta-step: 3 \newline
Task Variants: \(a_1 = 1\), \(a_2 \in [1, 2, 3, 4, 5]\) \\
\textbf{Evaluation Tasks} &
\((a_1, a_2)\) pairs: \newline
(4, 4), (4, 5), (5, 5), (6, 4) \\
\textbf{Loss \& Hyperparameters} &
\(\mathcal{L}_{total} = \lambda_{residual}\mathcal{L}_{residual} + \lambda_{data}\mathcal{L}_{data}\) \newline
\(\lambda_{residual} = 0.005,\quad \lambda_{data} = 1.0\) \\
\bottomrule
\end{tabular}
\label{tab:helm-exp-setup}
\end{table}
